# Supplementary material for: Average-reward model-free reinforcement learning: a systematic review and literature mapping
Source: arXiv:2010.08920 source file (2021-08-03)
Supplement: Supplementary file 1 [file appendix_abbrv_tbl.tex]

\begin{longtable}{p{0.15\textwidth}p{0.85\textwidth}}
\caption{Abbreviations.}
\label{tbl:abbreviation} \\
\endfirsthead

\multicolumn{2}{c}%
{{\tablename\ \thetable{} -- continued from previous page}} \\
\midrule[1pt]
\endhead

\hline
\multicolumn{2}{r}{{Continued on next page ...}} \\
\endfoot

\endlastfoot

\toprule[1pt]

AAPI & Adaptive Approximate Policy Iteration\\
AO-FTRL & Adaptive Optimistic Follow the Regularized Leader \\
\\
CSV & Constant Shifting Values \\
CVI & Contracting Value Iteration\\
\\
DP  & Dynamic Programming \\
DQN & Deep $Q_\gamma$-learning Neural-networks \\
\\
EEQL & Exploration Enhanced Q-Learning\\
\\
FIM & Fisher Information Matrix\\
\\
GARNET & Generic Average Reward Non-Stationary Environment Testbed\\
GPI &   Generalized Policy Iteration\\
\\
i.i.d & independent and indentically distributed \\
I2NAC & Implicit Incremental Natural Actor Critic\\
\\
KL & Kullback-Leibler\\
\\
LHS & Left Hand Side\\
LSPE & Least-Squares Policy Evaluation\\
LSPI & Least-Squares Policy Iteration\\
LSTD & Least-Squares Temporal Difference\\
\\
MDP &   Markov Decision Process\\
MSE & Mean Squared Error\\
MSPBE & Mean-Squared Projected Bellman Error\\
\\
NAC & Natural Actor Critic\\
NG & Natural Gradient\\
\\
ODE & Ordinary Differential Equation\\
OOMD & Optimistic Online Mirror Descent\\
\\
PI & Policy Iteration\\
POLITEX & Policy Iteration with Expert advice\\
PSRL & Posterior Sampling for Reinforcement Learning\\
\\
$Q_b$-learning & Q-learning with the average-reward optimality criterion \\
$Q_\gamma$-learning & Q-learning with the discounted-reward optimality criterion \\
\\
RHS & Right Hand Side\\
RL & Reinforcement Learning\\
RLSVI & Randomized Least-Squares Value Iteration\\
RM & Robbins-Monro, as in the RM algorithm \\
RVI & Relative Value Iteration\\
\\
SA & Stochastic Approximation\\
SGD & Stochastic Gradient Descent \\
SMART & Semi-Markov Average Reward Technique \\
SSP & Stochastic Shortest Path \\
\\
TD & Temporal Difference\\
\\
UCB & Upper Confidence Bound \\
UCRL & Upper Confidence Reinforcement Learning\\
\\
VI & Value Iteration\\

\bottomrule[1pt]
\end{longtable}
