# Supplementary material for: Average-reward model-free reinforcement learning: a systematic review and literature mapping
Source: arXiv:2010.08920 source file (2021-08-03)
Supplement: Supplementary file 2 [file appendix_glossary.tex]

\section{Glossary} \label{sec_glossary}
For the sake of clarity, we include the definition of some critical terminology used in this work.
Note that some terms in literature are vague and overloaded. %

\paragraph{Online vs offline learning:}
Online RL makes updates only with the experience from current interaction with the environment.
The experience is in the form of $\{ (s, a, s', r')_i \}_{i=1}^\xi$, where
$\xi$ indicates the batch size.
In contrast, offline (batch) RL utilizes previously collected data (from past interaction)
without additional online data collection \citep{levine_2020_offlinerl, fonteneau_2013_brl}.

\paragraph{Incremental vs batch updates:}
Incremental updates refer to per-step (step-wise) updates with batch size $\xi = 1$.
On the other hand, in batch updates, the batch size is typically $\xi \gg 1$.
By batches, we mean full-batches, unless specified otherwise as mini-batches.

\paragraph{Synchronous vs asynchronous updates:}
In synchronous settings, \emph{all} entries of the iterate are updated at each update iteration.
In asynchronous settings, only one (or some, but not all) of the entries is
updated at each update iteration.
Such an updated entry is the one that the agent visits.

\paragraph{On- vs off-policy learning:}
On-policy learning updates the learnable parameters associated to the behaviour policy
based on data collected using the same behaviour policy, which is being executed by the agent.
In other words, the data (experience) for learning is drawn from
the corresponding distribution under a policy that is also the target of learning.
Thus, the terms ``target'' and ``behaviour'' policies refer to the same policy.

On the other hand, off-policy learning updates the learnable parameters associated with
the target policy based on data collected using a different behaviour policy.
Thus, there are two distinct policies, namely target and behaviour policies.

\paragraph{Tabular vs function approximation settings:}
In tabular settings, the value function or the policy is represented by a look-up table,
where every state or every state-action pair has an entry.
This causes scalability problems in terms of memory, as well as
learning rate (too many entries to update).

A function approximator has a set of (learnable) parameters whose
size is typically much less than the number of tabular entries.
Hence, there exists generalization across states and actions.
Note that we may interpret the tabular setting as a special case of
\emph{linear} function approximation,
where there are as many (table-lookup) features as the tabel size.

\paragraph{Tabular $Q_b$-learning, $Q_\gamma$-learning, and Sarsa:}
\algref{alg:avgrew_qlearn_tabular} shows the general implementation of tabular $Q_b$-learning.
Its discounted-reward counterpart, \ie $Q_\gamma$-learning, can be obtained by
some appropriate changes regarding the use of discount factor $\gamma$ and the removal of $v_g^*$.
In \alglineref{alg:avgrew_qlearn_tabular}{line:deltafn}, the function $\Delta(\cdot)$
encodes the variations of $v_g^*$ approximation techniques discussed in \secref{sec:valiter_tabular}.
Both $Q_b$- and $Q_\gamma$-learning are VI-based and off-policy algorithms.

In contrast, the tabular Sarsa (\algref{alg:avgrew_sarsa_tabular}) is based on PI.
It operates on-policy; although one may argue that it has slight off-policy nature.

\begin{minipage}[t]{0.45\textwidth}
\vspace{0pt}
\begin{algorithm}[H]
\caption{Tabular $Q_b$-learning}
\label{alg:avgrew_qlearn_tabular}
\DontPrintSemicolon

IN: $\hat{q}_b^* \in \real{\setsize{S} \times \setsize{A}}, \beta_q, \beta_g$ \\
OUT: near-optimal policy \\
Initialize $\hat{q}_b^* \in \real{\setsize{S} \times \setsize{A}}$
    and $\hat{v}_g^* \in \real{}$. \\

\For{$t = 0, 1, \ldots, \tmaxhat$}{
    Observe the current state $s$. \\
    Choose an action $a$ with an exploration strategy,
        \eg $\epsilon$-greedy. \\ %
    Execute $a$. \\
    Observe $s'$ and $r'$. \\
    $\delta \gets
    r' + \max_{a' \in \setname{A}} \hat{q}_b^*(s', a')
        - \hat{v}_g^* - \hat{q}_b^*(s, a)$. \\
    $\hat{q}_b^*(s, a) \gets \hat{q}_b^*(s, a) + \beta_q \delta$. \\
    $\hat{v}_g^* \gets \hat{v}_g^* + \beta_g \Delta(s, a, s', r', \hat{q}_b^*, \hat{v}_g^*)$. \label{line:deltafn}\\

}
\end{algorithm}

\end{minipage}%
\hfill
\begin{minipage}[t]{0.45\textwidth}
\vspace{0pt}
\begin{algorithm}[H]
\caption{Tabular Sarsa (using $\hat{q}_b^\pi$)}
\label{alg:avgrew_sarsa_tabular}
\DontPrintSemicolon

IN: $\hat{q}_b^\pi \in \real{\setsize{S} \times \setsize{A}}, \beta_q, \beta_g$ \\
OUT: near-optimal policy \\
Initialize $\hat{q}_b^\pi \in \real{\setsize{S} \times \setsize{A}}$
    and $\hat{v}_g^\pi \in \real{}$ \\
Observe the current state $s$. \\
Choose $a$ based on $s$ and $\hat{q}_b^\pi$. \\
\For{$t = 0, 1, \ldots, \tmaxhat$}{
    Execute $a$. \\
    Observe $s'$ and $r'$ \\
    Choose $a'$ based on $s'$ and $\hat{q}_b^\pi$ with an exploration strategy,
    \eg $\epsilon$-greedy. \\
    $\delta \gets r' + \hat{q}_b^\pi(s', a') - \hat{v}_g^\pi - \hat{q}_b^\pi(s, a)$. \\
    $\hat{v}_g^\pi \gets \hat{v}_g^\pi + \beta_g \delta$. \\
    $\hat{q}_b^\pi(s, a) \gets \hat{q}_b^\pi(s, a) + \beta_q \delta$. \\
    $s \gets s'$ and $a \gets a'$.
}
\end{algorithm}

\end{minipage}
