# Supplementary material for: Average-reward model-free reinforcement learning: a systematic review and literature mapping
Source: arXiv:2010.08920 source file (2021-08-03)
Supplement: Supplementary file 3 [file appendix_notation_tbl.tex]

\begin{longtable}{p{0.17\textwidth}p{0.83\textwidth}}
\caption{Notations with the following conventions.
Scalars and scalar-valued functions are in light lower cases.
Vectors and vector-valued functions are in bold and lower cases.
Random variables are in light upper cases.
Matrices are in bold upper cases.
An overhead-symbol \emph{hat} denotes an approximation, \eg $\hat{v}_g^\pi \approx v_g^\pi$.
An \emph{asterisk} superscript denotes an optimal value, \eg the optimal policy $\pi^*$,
whereas a superscript $^\intercal$ denotes the transpose, as in $\vecb{v}^\intercal$.
}
\label{tbl:notation} \\
\endfirsthead

\multicolumn{2}{c}%
{{\tablename\ \thetable{} -- continued from previous page}} \\
\midrule[1pt]
\endhead

\hline \multicolumn{2}{r}{{Continued on next page ...}} \\
\endfoot

\endlastfoot

\midrule[1pt]

$\setname{T}, t$ &
The set of all discrete timesteps $t$ (stage, decision epoch), ie. $t \in \setname{T}$.
\\

$\tmax, \tmaxhat$ &
The final timestep is denoted by $\tmax$.
In infinite horizon, it is $\tmax = \infty$. \newline
The finite number of timesteps in experiments is $\tmaxhat \approx \tmax$.
\\

$t_{\sref}^\pi$ &
The timestep at which $\sref$ is visited while
following a policy~$\pi$, assuming that $\sref$ is recurrent under all policies.
\\

\midrule[1pt]

$\setname{S}, S$ &
The set of all states, ie. the state set $\setname{S}$. \newline
A random variable that takes on a value in $\setname{S}$ is denoted as $S$.
\\

$s, s', \sref$ &
A state instance (realization) or a state member of $\setname{S}$. \newline
Furthermore, $\sref$ represents a fixed reference state, and
$s'$ denotes a distinctly different state $s' \ne s$, or
the state at the next timestep, \ie $s' \eqdef s_{t+1}$.
\\

\midrule[1pt]

$\setname{A}, A$ &
The set of all actions, ie. the action set $\setname{A}$. \newline
A random variable that takes on a value in $\setname{A}$ is denoted as $A$.
\\

$a, a', \aref$ &
An action instance (realization) or an action member of $\setname{A}$. \newline
Furthermore, $\aref$ represents a fixed reference action, and
$a'$ denotes a distinctly different action $a' \ne a$, or
the action at the next timestep, \ie $a' \eqdef a_{t+1}$.
\\

\midrule[1pt]

$\setname{R}, R$ &
The set of all rewards, ie. the reward set $\setname{R}$. \newline
A random variable that takes on a value in $\setname{R}$ is denoted as $R$.
\\

$r, r'$ &
An reward instance (realization) or an reward member of $\setname{R}$. \newline
Furthermore, $r'$ denotes a distinctly different reward $r' \ne r$, or
the reward at the next timestep, \ie $r' \eqdef r_{t+1}$.
\\

$r(s, a, s')$ & %
A reward function $r_{sas}: \setname{S} \times \setname{A} \times \setname{S} \mapsto \real{}$
that outputs a reward given the current state $s$, current action $a$ and next state $s'$.
That is, $r(s_t, a_t, s_{t+1}) = \E{R_{t+1}}{ R_{t+1} | s_t, a_t, s_{t+1} }$.
\\

$r(s, a)$ &%
A reward function $r_{\mathsf{sa}}: \setname{S} \times \setname{A} \mapsto \real{}$,
where $r(s, a) = \E{S'}{r(s, a, S')}$.
\\

$r_\pi(s), \vecb{r}_\pi$ &
A reward function $r^\pi: \setname{S} \mapsto \real{}$,
where $r^\pi(s, a) = \E{A' \sim \pi}{r(s, A)}$. \newline
Stacking all possible rewards given all possible states $s$ yields a vector
$\vecb{r}_\pi \in \real{\setsize{S}}$.
\\

\midrule[1pt]
$\piset{}, \piset{SD}, \piset{SR}$ &
Set of all policies, ie. the policy set $\piset{}$. \newline
Its subsets include
the stationary and determinitic policy set $\piset{SD} \subset \piset{}$, and
the stationary and randomized policy set $\piset{SR} \subset \piset{}$.
\\

$\pi, \pi(a|s)$ &
A policy $\pi \in \piset{}$ that is a function
$\pi: \setname{S} \times \setname{A} \mapsto [0, 1]$.
Specifically, $\pi(a|s)$ denotes the probability of taking an action $a$
given the current state $s$.
\\

$\vecb{\theta}, \Theta$, \newline
$\pi(\vecb{\theta}), \pi_{\vecb{\theta}}$ &
A policy (actor) parameter vector and its set, \ie $\vecb{\theta} \in \Theta$;
\cf $\vecb{w} \in \setname{W}$ for critic. \newline
The parameterized policy is referred to as either $\pi(\vecb{\theta})$ or $\pi_{\vecb{\theta}}$.
\\

$\alpha$ &
Learning rate (step size, step length) used for updating $\vecb{\theta}$ for the actor.
\\

$\vecb{\phi}(s, a)$ &
A feature vector of the state-action pair $(s,a)$ for actor;
\cf $\vecb{f}(s,a)$ for critic.
\\

\midrule[1pt]

$v_g(\pi), v_g^\pi$ &
The expected average reward value of a policy, \ie $v_g^\pi \eqdef v_g(\pi)$.
It is also termed as stationary (steady state) reward, or simply the gain
(hence the subscript ``g'').
The gain of the optimal policy, \ie the optimal gain, is denoted by $v_g^* \eqdef v_g(\pi^*)$,
\\

$v_b(\pi, s)$, \newline
$v_b^\pi(s), \vecb{v}_b^\pi$ &
The relative state value of a policy, \ie $v_b^\pi(s) \eqdef v_b(\pi, s)$,
where the subscript ``b'' stands for bias.
Such value of the optimal policy is denoted by $v_b^* \eqdef v_b(\pi^*)$.
Stacking all states' relative values yields a vector
$\vecb{v}_b^\pi \in \real{\setsize{S}}$.
\\

$q_b(\pi, s, a)$, \newline
$q_b^\pi(s, a), \vecb{q}_b^\pi$ &
The relative state-action value of a policy, \ie $q_b^\pi(s, a) \eqdef q_b(\pi, s, a)$.
Such value of the optimal policy is denoted by $q_b^* \eqdef q_b(\pi^*)$.
Stacking all state-action relative values yields a vector
$\vecb{q}_b^\pi \in \real{\setsize{S} \setsize{A}}$.
\\

$\adv_b(\pi, s, a)$, \newline
$\adv_b^\pi(s, a), \vecb{\adv}_b^\pi$ &
The relative action advantage of a policy, \ie $\adv_b^\pi(s, a) \eqdef \adv_b(\pi, s, a)$.
Such advantage value of the optimal policy is denoted by $\adv_b^* \eqdef \adv_b(\pi^*)$.
Stacking all state-action relative values yields a vector
$\vecb{\adv}_b^\pi \in \real{\setsize{S} \setsize{A}}$.
\\

$\delta_{v_b}^\pi, \delta_{q_b}^\pi$ &
The relative TD on state value under a policy $\pi$ is denoted by $\delta_{v_b}^\pi(s, a, s')$,
whereas that on action value by $\delta_{q_b}^\pi(s, a, s', a')$.
\\

$\mathfrak{q}_b^\pi$, $\nu_b^\pi$ &
The surrogate action value, \ie
$\mathfrak{q}_b^\pi(s, a) \eqdef r(s, a) + \E{S_{t+1}}{v_b^\pi(S_{t+1})}$.
And the surrogate state value, \ie $\nu_b^\pi \eqdef v_b^\pi(s') + (v_g^\pi + \kappa)$
for some constant $\kappa \in \real{}$.
\\

$\vecb{w}, \setname{W}$, \newline
$\vecb{w}_v$, $\vecb{w}_q$, $\vecb{w}_{\adv}$, $\vecb{w}_g$ &
A value function parameter vector and its set, \ie $\vecb{w} \in \setname{W}$;
\cf $\vecb{\theta} \in \Theta$ for actor. \newline
Specific approximator's parameters for state and action values, as well as action advantages
are denoted by $\vecb{w}_v$, $\vecb{w}_q$, $\vecb{w}_{\adv}$, respectively.
\\

$\vecb{f}(s,a), \vecb{f}_{\vecb{\theta}}(s, a)$ &
A feature vector of the state-action pair $(s,a)$ for critic;
\cf $\vecb{\phi}(s,a)$ for actor. \newline
The $\vecb{\theta}$-compatible feature is defined as
$\vecb{f}_{\vecb{\theta}}(s, a) \eqdef \nabla \log \pi(a|s; \vecb{\theta})$.
\\

$\beta$ \newline
$\beta_g$, $\beta_v$, $\beta_q$, $\beta_{\adv}$ &
Learning rate (step size, step length) used for updating $\vecb{w}$ for the critic.
Specific approximator's learning rate for gain, state and action values, as well as action advantages
are denoted by $\beta_g$, $\beta_v$, $\beta_q$, and $\beta_{\adv}$, respectively.
\\

\midrule[1pt]

$p_\pi^\star(s)$ &
The unique stationary (steady-state) probability of state $s$ under a policy $\pi$.
\\

$p_\pi^\star(s, a)$ &
The unique stationary (steady-state) probability of a state-action pair $(s, a)$ under a policy $\pi$.
\\

$p(s'|s,a)$ &
The probability of going to the next state $s' \in \setname{S}$ given
the current state $s$ and the current action $a$.
\\

$\mat{P}_\pi$ &
The state transition stochastic matrix under a policy $\pi$.
Its size is of $\setsize{S}$-by-$\setsize{S}$.
\\

$\isd$ &
The initial state distribution, $S_0 \sim \isd$.
\\

$\mat{D}_\pi^\star$ &
A diagonal $\setsize{S}$-by-$\setsize{S}$ matrix with
$p_\pi^\star(s), \forall s \in \setname{S}$ in its diagonal.
\\
\midrule[1pt]

$\vecb{e}, \vecb{e}_{\vecb{\theta}}, \vecb{e}_{\vecb{w}}$ &
An eligibility trace vector is denoted by $\vecb{e}$.
Specifically, $\vecb{e}_{\vecb{\theta}}$ is used for the actor's $\vecb{\theta}$ updates,
whereas $\vecb{e}_{\vecb{w}}$ for the critic's $\vecb{w}$ updates.
\\

$\vecb{F}_{a}(\vecb{\theta})$ &
The Fisher (information) matrix based on action distribution,
\ie a parameterized policy $\pi(\vecb{\theta})$.
It is $\vecb{F}_{a} \in \real{\dim(\vecb{\theta}) \times \dim(\vecb{\theta})}$.
\\

$\vecb{F}_{sa}(\vecb{\theta})$ &
The Fisher (information) matrix based on state-action distribution induced by
a parameterized policy $\pi(\vecb{\theta})$,
\ie $p(s, a; \vecb{\theta})$.
It is $\vecb{F}_{sa} \in \real{\dim(\vecb{\theta}) \times \dim(\vecb{\theta})}$.
\\

\midrule[1pt]

$\lambda$ &
A trace decay factor $0 < \lambda < 1$. %
\\

$\gamma, \gammabw$ &
A discount factor $0 < \gamma < 1$.
The Blackwell's discount factor is denoted by $\gammabw$.
\\

$\varepsilon$ &
Some positive error or some convergence tolerance, used for, \newline
\eg termination of an iterative procedure.
\\

$\epsilon$ &
The probability of selecting a non-greedy action, $\epsilon \in [0, 1]$, as in \newline
$\epsilon$-greedy exploration, $\epsilon$-soft policy.
\\

$\kappa$ &
Some positive constant.
\\

$\xi$ &
Some positive batch size.
\\

$d$ &
The number of dimensions,
\eg a vector $\vecb{v} \in \real{3}$ has $d_{\vecb{v}} = 3$.
\\

\midrule[1pt]

$\mathbb{B}^\pi, \mathbb{B}^*$ &
The Bellman operators, where
$\mathbb{B}^\pi$ denotes the Bellman policy expectation operator, whereas
$\mathbb{B}^*$ the Bellman optimality operator.
\\

$\mathbb{E}$ &
The expectation operator.
\\

$\mathbb{P}$ &
Some projection operator.
\\

$\real{}$ &
The set of real numbers.
\\

$\integer{}$, $\integer{\ge 0}$ &
The set of integer numbers $\integer{}$, whereas
$\integer{\ge 0}$ indicates non-negative integers.
\\

\midrule[1pt]

$\prob{X = x}$ &
The probability that a random variable $X$ has a value $x$.
\\

$\nabla$ &
The gradients, \ie $\nabla \eqdef \partdiff{\vecb{\theta}}$,
as in $\nabla v_g(\vecb{\theta}) \in \real{\dim(\vecb{\theta})}$.
\\

\bottomrule[1pt]
\end{longtable}
