# Supplementary material for: Average-reward model-free reinforcement learning: a systematic review and literature mapping
Source: arXiv:2010.08920 source file (2021-08-03)
Supplement: Supplementary file 4 [file appendix_tbl_politerwork_evaloff.tex]

\midrule[1pt]
\textbf{Work \steppoliterworkcounter~(EI)} &
\textbf{\cite{murphy_2016_batch}} \\*
Contribution &
Arguably the first off-policy, batch, actor-critic algorithm.
\\*
Experiment &
On mobile health
\\*

\midrule[1pt]
\textbf{Work \steppoliterworkcounter~(E)} &
\textbf{\cite{liu_2018_offpol, mousavi_2020_offpol, tang_2020_doubly}} \\*
Contribution &
Off-policy value-function estimation by applying importance sampling on
the average visitation distribution of single steps
of state-action pairs (instead of the much higher dimensional distribution
of whole trajectories).
Thus, decreasing the variance because it avoid the cumulative product across time
in the \emph{density ratio}, and eliminating the estimator's dependence on the horizon.
A mini-max loss function for estimating the density ratio of two stationary state distributions,
with trajectories sampled from only the behavior distribution.
A closed-form solution for the case of RKHS.
\\*
Experiment &
Taxi (discrete action and state spaces, modified to be infinite horizon),
Pendulum (continuous states and actions),
SUMO Traffic Simulator,
The proposed method generally outperforms the standard trajectory-wise and step-wise WIS,
and works favorably in long-horizon problems.
\\*

\midrule[1pt]
\textbf{Work \steppoliterworkcounter~(E:off)} &
\textbf{} \\*
GenDICE: Generalized Offline Estimation of Stationary Values
Ruiyi Zhang, Bo Dai, Lihong Li, Dale Schuurmans

Contribution &
GenDICE, for GENeralized stationary DIstribution Correction Estimation.
consistent estimation of quantities defined by the stationary distribution
    Behavior-agnostic Off-Policy Evaluation

recast OPE as estimating a correction ratio function,
which significantly alleviates variance.

based on estimating a ratio that corrects for the discrepancy between the stationary and em-
pirical distributions, derived from fundamental properties of the stationary distri-
bution, and exploiting constraint reformulations based on variational divergence
minimization.

prove its consistency under general conditions, provide an error analysis,

\\*
Experiment &
and demonstrate strong empirical performance on benchmark problems, including
off-line PageRank and off-policy policy evaluation

compare to Liu et al. (2018) (referred to as “IPS” here) in the Taxi domain with a learned
behavior policy1
 Evaluation with Taxi

 n three control tasks: a discrete-control task Cartpole and
two continuous-control tasks Reacher and HalfCheetah
    BUT discounted reward case
\\*

RWORK
only published algorithm in the literature, to the best of our knowledge, that solves agnostic-behavior
off-policy evaluation is DualDICE (Nachum et al., 2019). However, DualDICE was developed
discounted problems and its results become unstable when the discount factor approaches 1 (see
below). By contrast, GenDICE can cope with the more challenging problem of undiscounted reward
estimation in the general behavior-agnostic setting.

\midrule[1pt]
\textbf{Work \steppoliterworkcounter~(E:off)} &
\textbf{\cite{}} \\*
A maximum-entropy approach to off-policy evaluation in average-reward MDPs
Nevena Lazić

Contribution &
first finite-sample OPE error bound on gain estimation (batch, off-policy)
    depend on the MDP mixing time

a maximum-entropy approach to
finding stationary distributions with function approximation
    note that the maximum-entropy objective corresponds to minimizing the KL-
    divergence between the target distribution and the uniform distribution
 batch policy evaluation
\\*
Experiment &
Synthetic environments. We generate synthetic MDPs with 100 states, 10 actions, and transition
matrices P generated by sampling entries uniformly at random and normalizing columns to sum to

OpenAI Gym environments [Brockman et al., 2016] (Taxi and Acrobot)
Linear quadratic regulator

Acrobot: episodic
    after which we reset

compute the true
policy values Jπ using Monte-Carlo simulation for Acrobot, and exactly for other environmen
\\*

MDPs that
are ergodic and linear (i.e. where rewards and dynamics are linear in some known
features)
 non-i.i.d. data (coming from a single trajectory)

me: becomes like model-based
    as estimating M: transition matrix, eq 11

RWORK:
Most recent state-of-the-art
OPE methods for this setting estimate the ratios of stationary distributions of the target and behavior
policy [Liu et al., 2018, Nachum et al., 2019a, Wen et al., 2020, Nachum and Dai, 2020].

\midrule[1pt]
\textbf{Work \steppoliterworkcounter~(E:off)} &
\textbf{\cite{zhang_2021_gtd}} \\*
Contribution &
Gradient TD to off-policy poleval with fn approximator, resulting in
the first convergent off-policy linear function approximation algorithms for
estimating gain and bias.
No need for estimating the density ratio.
not suffer from deadly triad, althoguh all 3 present.
a) One- Stage Differential Gradient Q Evaluation (Diff-GQ1, \equ{9, 11}) based on
the first regularized MSPBE, and exploits Fenchel’s duality,
no need for gain estimate.
b) Two-Stage Differential Gradient Q Evaluation (Diff-GQ2),
not require Assumption 4.1, with 2nd regularized MSPBE2, and exploits Fenchel’s duality,
with paramerized gain due to parameterized state values.
And their projected versions.
As GTD, it has 2 learnable param vectors.
\\*
Experiment &
Evaluate the gain.
a) On Boyan chain (with a nonzero reward for each action) and Linear Function Approximation.
All proposal outperform GradientDICE (the density-ratio-based algorithm).
b) On Mujoco (HalfCheetah, Walker2d, Hopper, Swimmer) and Nonlinear Function Approximation
Diff-GQ1 consistently per- forms the best.
\\*
