# Supplementary material for: Average-reward model-free reinforcement learning: a systematic review and literature mapping
Source: arXiv:2010.08920 source file (2021-08-03)
Supplement: Supplementary file 5 [file appendix_glossary_qlearn.tex]

\begin{algorithm}[H]
\caption{Tabular $Q_b$-learning}
\label{alg:avgrew_qlearn_tabular}
\DontPrintSemicolon

IN: $\hat{q}_b^* \in \real{\setsize{S} \times \setsize{A}}, \beta_q, \beta_g$ \\
OUT: near-optimal policy \\
Initialize $\hat{q}_b^* \in \real{\setsize{S} \times \setsize{A}}$
    and $\hat{v}_g^* \in \real{}$. \\

\For{$t = 0, 1, \ldots, \tmaxhat$}{
    Observe the current state $s$. \\
    Choose an action $a$ with an exploration strategy,
        \eg $\epsilon$-greedy. \\ %
    Execute $a$. \\
    Observe $s'$ and $r'$. \\
    $\delta \gets
    r' + \max_{a' \in \setname{A}} \hat{q}_b^*(s', a')
        - \hat{v}_g^* - \hat{q}_b^*(s, a)$. \\
    $\hat{q}_b^*(s, a) \gets \hat{q}_b^*(s, a) + \beta_q \delta$. \\
    $\hat{v}_g^* \gets \hat{v}_g^* + \beta_g \Delta(s, a, s', r', \hat{q}_b^*, \hat{v}_g^*)$. \label{line:deltafn}\\

}
\end{algorithm}
