# Supplementary material for: Average-reward model-free reinforcement learning: a systematic review and literature mapping
Source: arXiv:2010.08920 source file (2021-08-03)
Supplement: Supplementary file 6 [file appendix_glossary_sarsa.tex]

\begin{algorithm}[H]
\caption{Tabular Sarsa (using $\hat{q}_b^\pi$)}
\label{alg:avgrew_sarsa_tabular}
\DontPrintSemicolon

IN: $\hat{q}_b^\pi \in \real{\setsize{S} \times \setsize{A}}, \beta_q, \beta_g$ \\
OUT: near-optimal policy \\
Initialize $\hat{q}_b^\pi \in \real{\setsize{S} \times \setsize{A}}$
    and $\hat{v}_g^\pi \in \real{}$ \\
Observe the current state $s$. \\
Choose $a$ based on $s$ and $\hat{q}_b^\pi$. \\
\For{$t = 0, 1, \ldots, \tmaxhat$}{
    Execute $a$. \\
    Observe $s'$ and $r'$ \\
    Choose $a'$ based on $s'$ and $\hat{q}_b^\pi$ with an exploration strategy,
    \eg $\epsilon$-greedy. \\
    $\delta \gets r' + \hat{q}_b^\pi(s', a') - \hat{v}_g^\pi - \hat{q}_b^\pi(s, a)$. \\
    $\hat{v}_g^\pi \gets \hat{v}_g^\pi + \beta_g \delta$. \\
    $\hat{q}_b^\pi(s, a) \gets \hat{q}_b^\pi(s, a) + \beta_q \delta$. \\
    $s \gets s'$ and $a \gets a'$.
}
\end{algorithm}
